# Supplementary material for: Black-Box Verification for GUI Applications
Source: arXiv:1210.4686 source file (2012-10-17)
Supplement: Supplementary file 1 [file appendix.tex]

\newpage
\begin{appendix}

\section{Overview of our Approach}

\begin{figure}
	\centering
	\includegraphics[width=\textwidth]{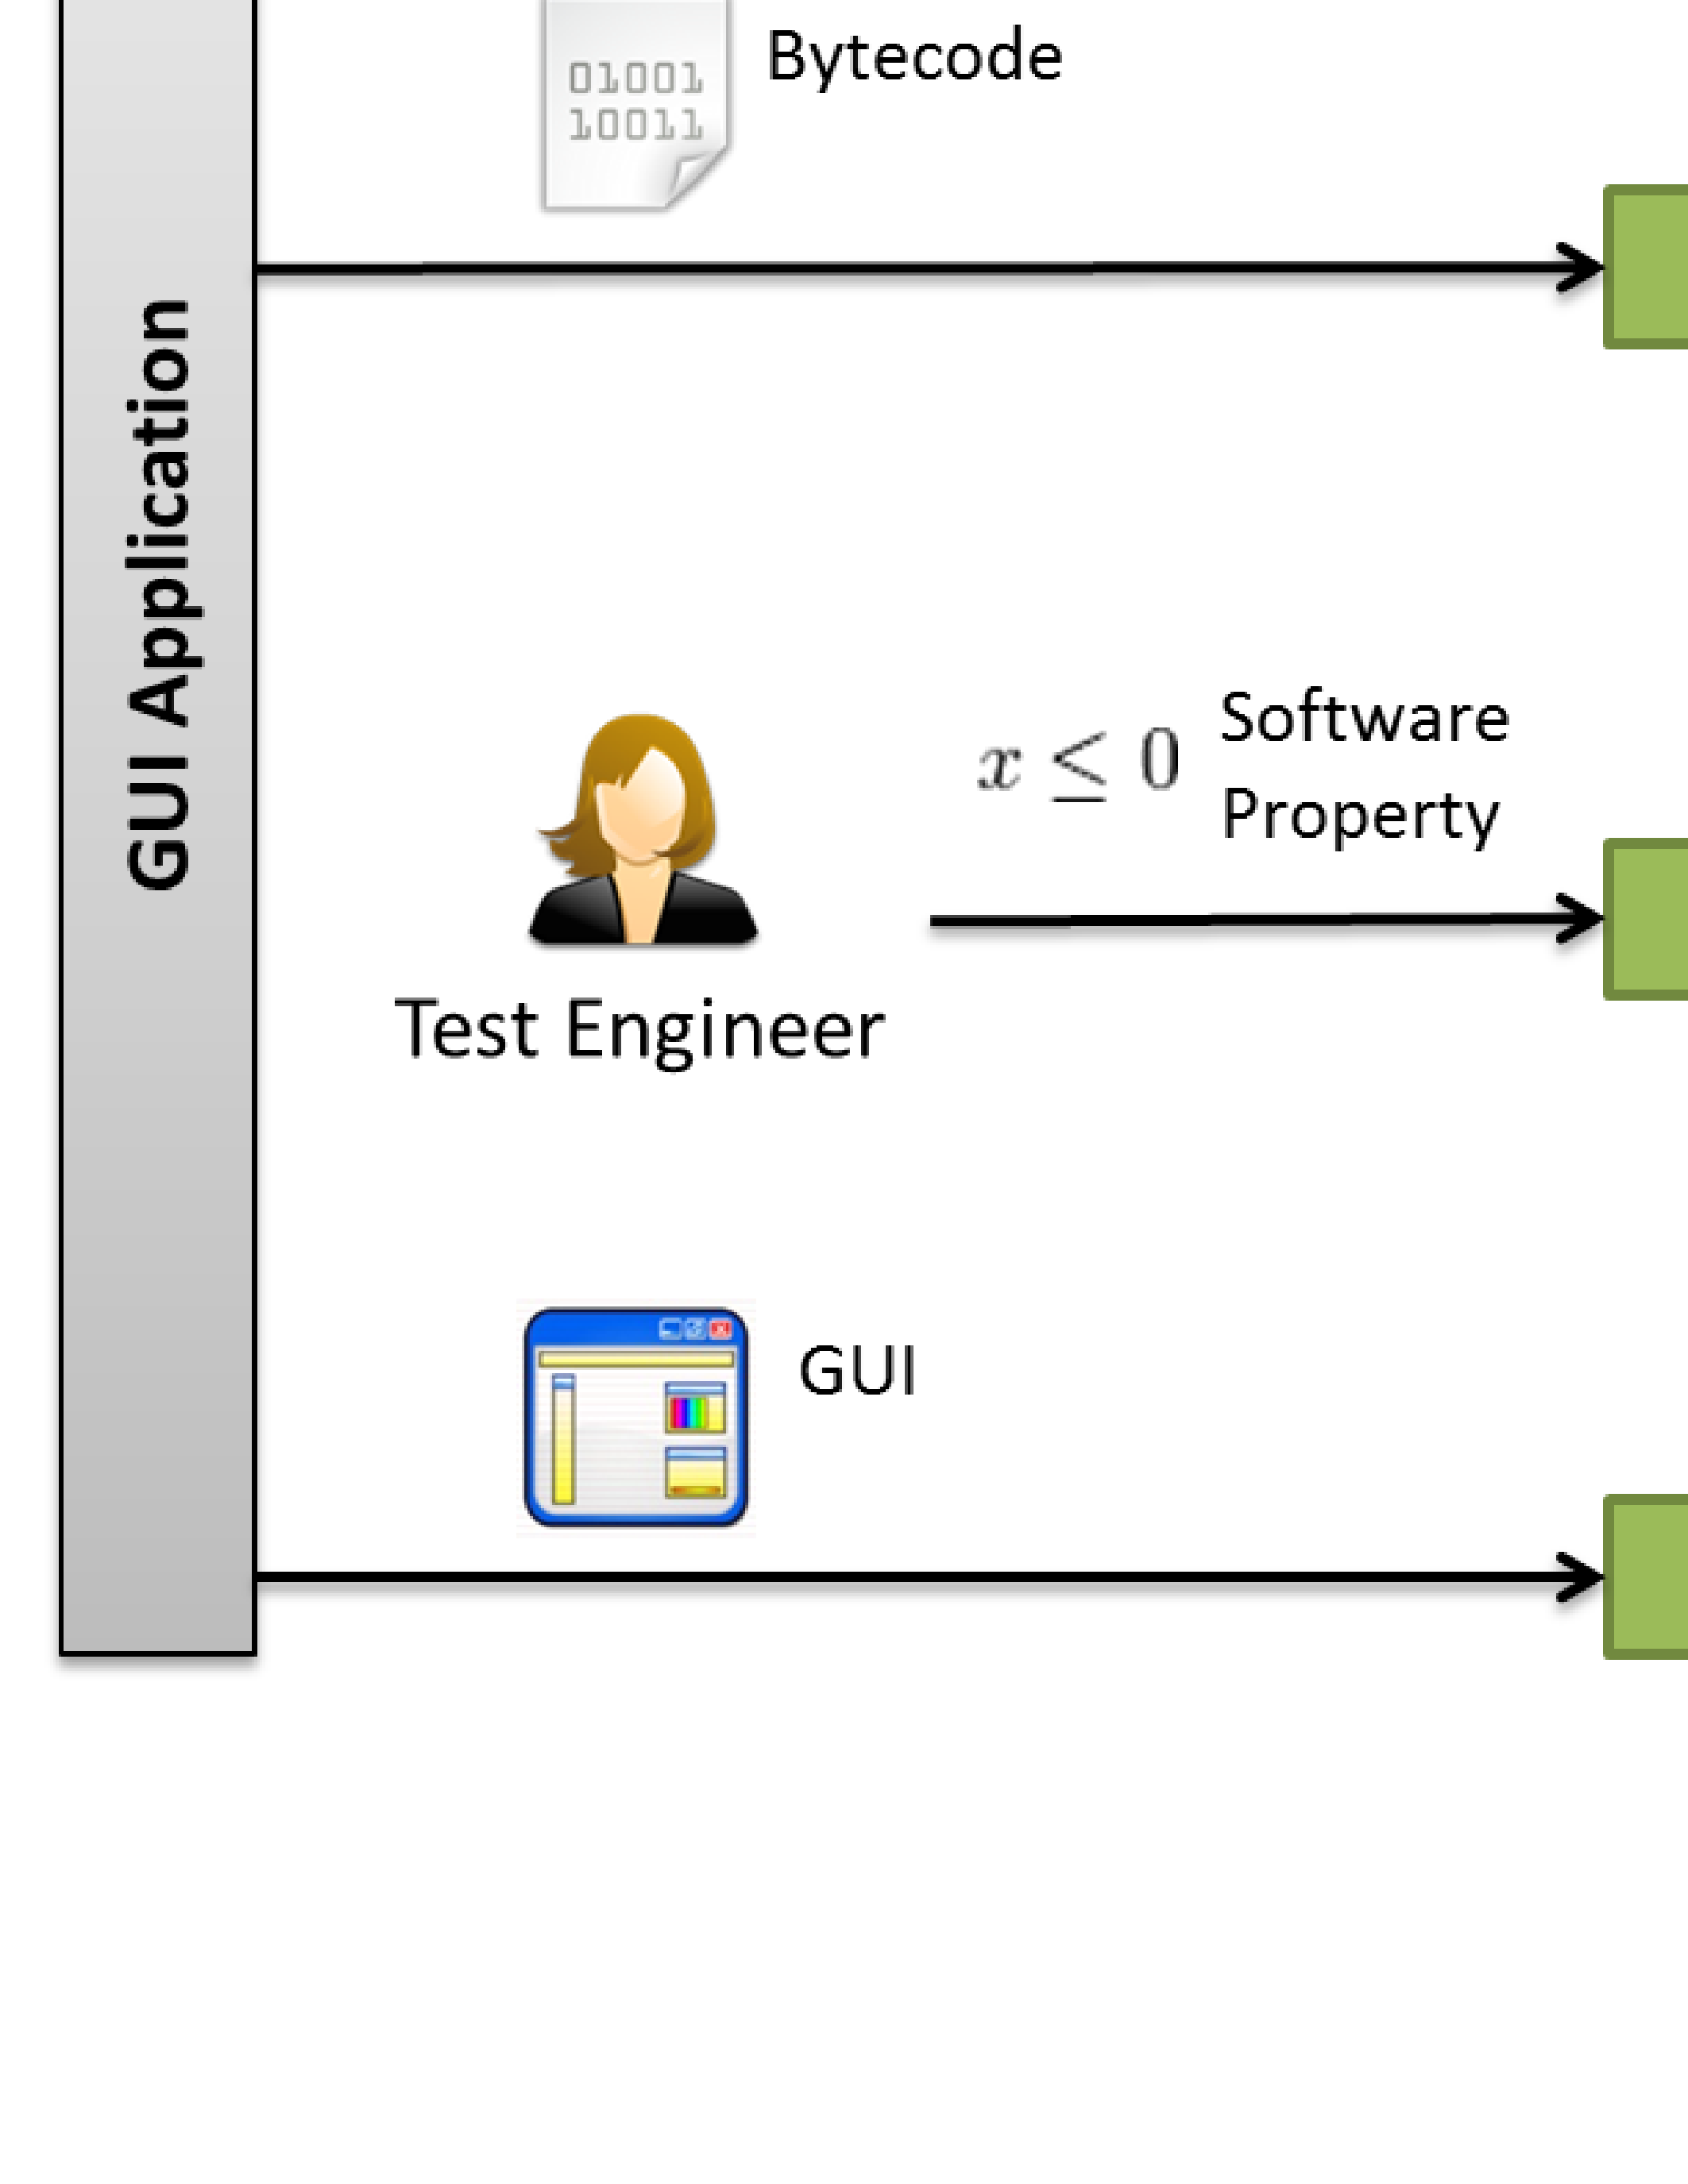}
	\caption{Overview of our Approach.}
	\label{fig:approach}
\end{figure}

\end{appendix}
